# Supplementary material for: Fact-Checking with Contextual Narratives: Leveraging Retrieval-Augmented LLMs for Social Media Analysis
Source: arXiv:2504.10166 source file (2025-07-22)
Supplement: Supplementary file 1 [file additional_figures.pdf]

# Additional Figures for Fact-Checking with Contextual Narratives: Leveraging Retrieval-Augmented LLMs for Social Media Analysis

April 10, 2025

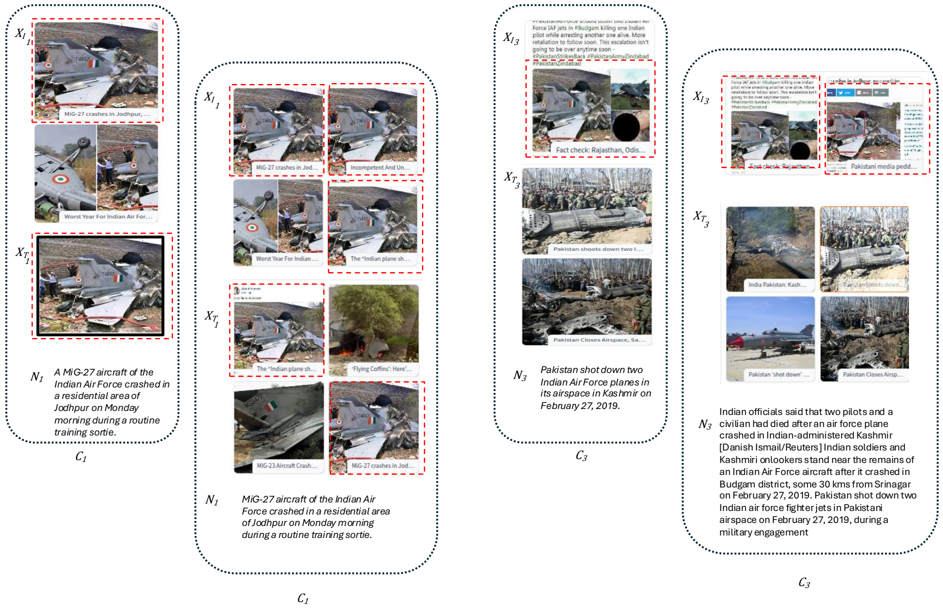


Figure 1: Overview of Cluster Refinement: Individual Cluster Refinements lead to discovery of evidence to strengthen the Narrative of a cluster. This also leads to more relevant evidence for the final step of judgment. In the background are the initial clusters, in the foreground are refined clusters with more relevant evidence.

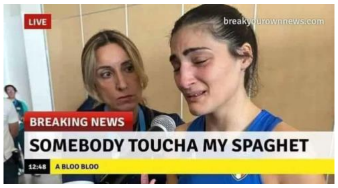


**Story: The International Boxing Association will award Angela Carini prize money equivalent to an Olympic champion despite her abandoning her fight against Algerias Imane Khelif**

**Please answer the following questions:**

How comprehensive is the fact-checker's explanation in addressing all the key facts from the Story?
1 - Not at all comprehensive
3 - Covers most key facts
5 - Fully comprehensive

How clear is the fact-checker's explanation?
1 - Not clear at all
3 - Fairly clear
5 - Very clear and intuitive

**Read these Key Facts Related to Story**

- The evidence text is unrelated to the claim
- Fig 32 Common Logical Fallacies Infographic with the name and description of eight logical fallacies Logical fallacies Red Herring Stating an unrelated point instead of addressing the argument Anecdotal Evidence Refuting systematic evidence with individual counterexamples Division Assuming that what is true of a group is true for each of its individual members Ad Hominem Attacking the person instead of their claim Confirmation Bias Ignoring evidence that contradicts your claim Anonymous Authority Relying on the claims of an unnamed expert as evidence Slippery Slope Claiming that a small first step will result in extreme subsequent events Sweeping Generalizations Applying a general rule incorrectly to specific cases Logical fallacies are identified as errors in reasoning that can undermine arguments including examples such as Red Herring Anecdotal Evidence and Ad Hominem
- articleimage Angela Carini abandoned her fight against Imane Khelif at the Paris Olympics 2024 after just 46 seconds in the first round due to a heavy punch
- Italian boxer Angela Carini to be awarded prize money by IBA despite Olympic defeat to Algerias Imane Khelif Italian boxer Angela Carini to be awarded prize money by IBA despite Olympic defeat to Algerias Imane Khelif The International Boxing Association will award Angela Carini prize money equivalent to an Olympic champion despite her Olympic defeat to Algerias Imane Khelif

**A fact checker thinks this story is True Claim**

**Explanation by Fact Checker**

Fact 4 contains Relevant Reverse Search Evidence that supports the claim The summary mentions the International Boxing Association awarding Angela Carini a goldmedal style bonus after she abandoned her bout against Algerias Imane Khelif which aligns with the claim The Location International Boxing Association Named Person Angela Carini Imane Khelif and Main Topic awarding prize money despite abandoning the fight all support the claim No conflicts were found in the evidence

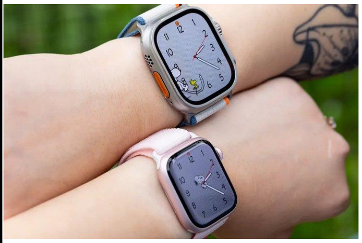

**Story: The latest Apple Watch has been banned in the United States due to a patent dispute**

**Please answer the following questions:**

How comprehensive is the fact-checker's explanation in addressing all the key facts from the Story?
1 - Not at all comprehensive
3 - Covers most key facts
5 - Fully comprehensive

How clear is the fact-checker's explanation?
1 - Not clear at all
3 - Fairly clear
5 - Very clear and intuitive

**Read these Key Facts Related to Story**

1. Patent infringement may ban Apple from selling watches in the US Patent infringement may ban Apple from selling watches in the US 1 The US International Trade Commission ITC found that Apples devices infringe upon the patent rights of Masimo which may ban Apple from selling watches in the US pending presidential approval and potential appeals in court
2. Apple watch on sale 11 series Apple watch on sale 11 series is available for delivery to addresses within other countries
3. The evidence text is unrelated to the claim
4. Apple announced that it will halt sales of the Apple Watch Series 9 and Apple Watch Ultra 2 in the United States starting December 21 due to an ITC ruling related to a patent dispute with Masimo over blood oxygen sensor technology

**A fact checker thinks this story is Misleading**

**Explanation by Fact Checker**

The claim states that the latest Apple Watch has been banned in the United States due to a patent dispute Fact 4s provides evidence that Apple will pause selling the Series 9 and Ultra 2 starting December 21st due to an ITC import ban following a patent dispute with Masimo over its SpO2 sensor in the United States However this does not confirm a complete ban on the latest Apple Watch in the United States as the claim suggests The evidence indicates a pause in sales for specific models not a total ban Therefore the claim is misleading as it overstates the situation Other Facts either do not provide relevant evidence or conflict with the claim by indicating availability of Apple Watches in other regions

Figure 2: User Study 1 : Comprehensiveness and Clarity scores for Explanations

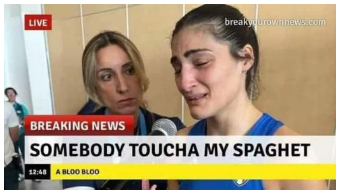


**Story: The International Boxing Association will award Angela Carini prize money equivalent to an Olympic champion despite her abandoning her fight against Algerias Imane Khelif**

**This story is True**

**Explanation by Users**

1. For additional context The International Boxing Association IBA is not associated with the Olympics The International Olympic Committee IOC revoked the IBAs recognition in 2023 due to concerns about governance financial mismanagement and other issues
2. Note Needed The awarding of this prize money confirms the IOCs issues about corruption and impartiality Proven by IBA President Umar Kremlev using AntiLGBT rhetoric to justify the decision The IBA are officially no longer the sports world governing bo

**Explanation by Fact Checker**

Source 4 contains Relevant Reverse Search Evidence that supports the claim The summary mentions the International Boxing Association awarding Angela Carini a goldmedal style bonus after she abandoned her bout against Algerias Imane Khelif which aligns with the claim The Location International Boxing Association Named Person Angela Carini Imane Khelif and Main Topic awarding prize money despite abandoning the fight all support the claim No conflicts were found in the evidence

**Sources used by the Fact Checker:**

1. The evidence text is unrelated to the claim
2. Fig 32 Common Logical Fallacies Infographic with the name and description of eight logical fallacies Logical fallacies Red Herring Stating an unrelated point instead of addressing the argument Anecdotal Evidence Refuting systematic evidence with individual counterexamples Division Assuming that what is true of a group is true for each of its individual members Ad Hominem Attacking the person instead of their claim Confirmation Bias Ignoring evidence that contradicts your claim Anonymous Authority Relying on the claims of an unnamed expert as evidence Slippery Slope Claiming that a small first step will result in extreme subsequent events Sweeping Generalizations Applying a general rule incorrectly to specific cases Logical fallacies are identified as errors in reasoning that can undermine arguments including examples such as Red Herring Anecdotal Evidence and Ad Hominem
3. articleimage Angela Carini abandoned her fight against Imane Khelif at the Paris Olympics 2024 after just 46 seconds in the first round due to a heavy punch
4. Italian boxer Angela Carini to be awarded prize money by IBA despite Olympic defeat to Algerias Imane Khelif Italian boxer Angela Carini to be awarded prize money by IBA despite Olympic defeat to Algerias Imane Khelif The International Boxing Association will award Angela Carini prize money equivalent to an Olympic champion despite her Olympic defeat to Algerias Imane Khelif

***Task Instructions***
*You are presented with a news story that has already been fact-checked. Two different explanations are provided:*
*•**Explanation by Users:** How users evaluated the claim.*
*•**Explanation by Fact-Checker:** How a fact-checker justified their verdict.*
***Your Task:** Select which explanation is better based on:*
*•How intuitive the explanation is*
*•How clear and concise it is*
*•How well it supports the given ground truth label of the story (e.g., True or Misleading)*
*Please read both explanations carefully before making your selection.*

**Please answer the following question:**
Which explanation is more intuitive, clear, and better supports the story being labeled as **True**?
1 – Users 2 - Fact Checker

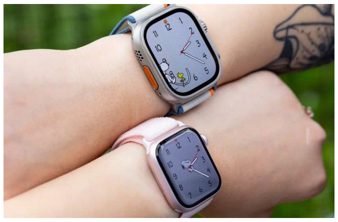

**Story: The latest Apple Watch has been banned in the United States due to a patent dispute**

**This story is Misleading**

**Explanation by Users**

1. Due to the infringement of an oximeter patent the US International Trade commission has ordered halting of Apple Watch series 9 and Apple Watch Ultra 2 sales by Christmas Apple may be able to resolve this via a software update and NO current devices are affected
2. The ban is solely due to a patent dispute Apple is facing after the US International Trade Commission ruled that they infringed on patents for pulse oximetry tech made by Masimo The ban starts December 24 and only affects the Watch 9 Series amp Ultra 2 Source Associated Press
3. The Apple Watch Series 9 and Ultra 2 are not getting banned they are just suspending sales

**Explanation by Fact Checker**

The claim states that the latest Apple Watch has been banned in the United States due to a patent dispute Source 4s provides evidence that Apple will pause selling the Series 9 and Ultra 2 starting December 21st due to an ITC import ban following a patent dispute with Masimo over its SpO2 sensor in the United States However this does not confirm a complete ban on the latest Apple Watch in the United States as the claim suggests The evidence indicates a pause in sales for specific models not a total ban Therefore the claim is misleading as it overstates the situation Other Sources either do not provide relevant evidence or conflict with the claim by indicating availability of Apple Watches in other regions

**Sources used by the Fact Checker:**

1. Patent infringement may ban Apple from selling watches in the US Patent infringement may ban Apple from selling watches in the US 1 The US International Trade Commission ITC found that Apples devices infringe upon the patent rights of Masimo which may ban Apple from selling watches in the US pending presidential approval and potential appeals in court
2. Apple watch on sale 11 series Apple watch on sale 11 series is available for delivery to addresses within other countries
3. The evidence text is unrelated to the claim
4. Apple announced that it will halt sales of the Apple Watch Series 9 and Apple Watch Ultra 2 in the United States starting December 21 due to an ITC ruling related to a patent dispute with Masimo over blood oxygen sensor technology

***Task Instructions***
*You are presented with a news story that has already been fact-checked. Two different explanations are provided:*
*•**Explanation by Users:** How users evaluated the claim.*
*•**Explanation by Fact-Checker:** How a fact-checker justified their verdict.*
***Your Task:** Select which explanation is better based on:*
*•How intuitive the explanation is*
*•How clear and concise it is*
*•How well it supports the given ground truth label of the story (e.g., True or Misleading)*
*Please read both explanations carefully before making your selection.*

**Please answer the following question:**
Which explanation is more intuitive, clear, and better supports the story being labeled as **Misleading**?
1 – Users 2 - Fact Checker

Figure 3: User Study 2: Preference between Explanation by Users(Notes) and Explanations by FactChecker (CRAVE)
